# Supplementary material for: Learn-to-Score: Efficient 3D Scene Exploration by Predicting View Utility
Source: arXiv:1806.10354 ancillary file (2018-07-31)
Supplement: Supplementary file 1 [file supplementary_material.pdf]

# Learn-to-Score: Efficient 3D Scene Exploration by Predicting View Utility Supplementary Material

Benjamin Hepp<sup>1,2</sup>, Debadeepta Dey<sup>2</sup>, Sudipta N. Sinha<sup>2</sup>,  
Ashish Kapoor<sup>2</sup>, Neel Joshi<sup>2</sup>, and Otmar Hilliges<sup>1</sup>

<sup>1</sup> ETH Zurich

<sup>2</sup> Microsoft Research

In Section 1, we present more details about the problem formulation and in section 2 more details on 3D scene exploration are provided. Section 3 provides enlarged versions of the performance plots from the main paper. Next, in Section 4, we show an extended evaluation of hyperparameters in our model. In Section 5, we visualize slices of the multi-scale representation of the occupancy map for different grid sizes. Following this, in Section 6, we give additional details on the training procedure. We finish with Section 7 by discussing how our approach relates to Partially Observable Markov Decision Processes (POMDPs) and their solution methods.

## 1 Details on world model and exploration

As discussed in the main text we model the world as a uniform voxel grid  $V$  where each voxel  $v \in V$  has a position  $v^p \in W$ , where  $W = [w^{min}, w^{max}]$  is the world bounding box.

At each time-step  $t_i, i \geq 0$  of an episode we add new viewpoints to the candidate set. The new viewpoints are those neighbors of the current camera pose which do not lead to a collision and stay within the world bounding box. A collision occurs if a bounding box of size  $(1m, 1m, 1m)$  centered at the camera pose intersects with any occupied or unknown voxel or if a ray shot from the current camera pose to the new camera pose intersects with any occupied or unknown voxel. The neighbors of a viewpoint are defined by the following local movements:

- Move forward by  $2.5m$
- Move backward by  $2.5m$
- Move left by  $2.5m$
- Move right by  $2.5m$
- Move up by  $2.5m$
- Move down by  $2.5m$
- Rotate yaw clockwise by  $25^\circ$
- Rotate yaw counter-clockwise by  $25^\circ$
- Rotate yaw by  $180^\circ$

When updating the state of voxels we clamp occupancy values to the range  $[occ^{lo}, occ^{hi}]$  with  $occ^{lo} = 0.12$  and  $occ^{hi} = 0.97$  as in [1]. The voxel uncertainty is updated by keeping an internal observation count  $M^n(v)$  for each voxel that is increased by one each

time a ray intersects the voxel. The uncertainty is then defined as

$$M^o(v) = \exp(-\eta M^n(v)) \quad . \quad (1)$$

To enable initial movement of the camera we clear a bounding box  $B = [(-3m, -3m, -3m), (3m, 3m, 3m)]$  around the initial camera position by setting  $M_{t_0}^o(v)(t_0) = occ^{lo}$ ,  $M_{t_0}^n(v) = 1/\eta \forall v \in V$  with  $v^p \in B$ .

When running episodes we only consider viewpoint candidates that have been visited less than 2 times to prevent visiting viewpoints too often and incentivising a faster exploration. We use this heuristic for all methods, including the oracle. A kd-tree is used to keep track of the number of visited poses (using both the location and orientation quaternion).

## 2 Details on 3D Scene Exploration

Throughout this work we use a pinhole camera model with 64 horizontal and vertical pixels, a field of view of  $90^\circ$  and a maximum ray distance of  $10m$ . Note that the ray distance is chosen such that the diameter of the projection cone of a pixel spans less than one voxel at the maximum ray distance.

To update the state of the voxels we take each ray described by the depth image and iterate through all intersecting voxels starting from the projection center (see Fig. 1 of the main text). Voxel uncertainties are updated as described in Sec. 4.1 of the main text with  $\eta = \frac{1}{2}$ .

As mentioned in the main text we assume that the utility function is submodular. This allows us to perform lazy evaluations of the utility function [2]: We keep a list of viewpoints sorted by decreasing score. After an update of the map we recompute the score for the viewpoint at the start of the list. If the new score is lower than the score of the following viewpoint in the list we move the viewpoint back in the list until the list is sorted again. We repeat this step until the first viewpoint has a higher score than the following viewpoint in the list. Because the viewpoint scores can only decrease with a map update (submodular property) this guarantees that at the end the highest scoring viewpoint is at the front of the list. This strategy typically allows us to only evaluate about 10 viewpoints per step instead of on the order of 100 or 1000 viewpoints.

## 3 Enlarged performance plots

In Fig. Fig. 1 and Fig. Fig. 2 we show enlarged versions of the plots from the main manuscript showing observed surface voxels vs. time for all methods.

## 4 Extended evaluation

We identify the following hyperparameters that we can choose for our model:

- *Input channels*: Input channels to use from the occupancy map
- *Input scales*: Which scales to use for the multi-scale representation

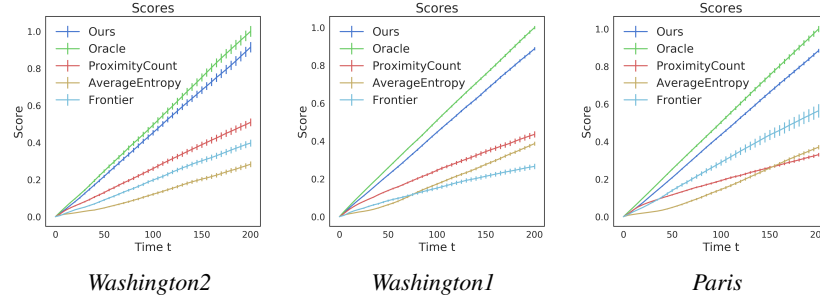

Fig. 1: Plot of observed surface voxels vs. time for all methods on the *Washington2*, *Washington1* and *Paris* scene. Plots were computed across 50 explorations. Best viewed in color.

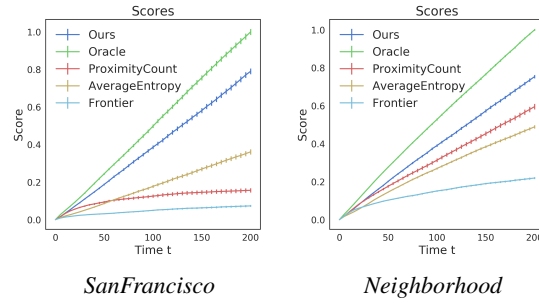

Fig. 2: Plot of observed surface voxels vs. time for all methods on the *SanFrancisco* and *Neighborhood* scene. Plots were computed across 50 explorations. Best viewed in color.

- $N_u$ : Number of units per block
- $N_f$ : Number of added features per unit
- $N_{h1}$ : Number of hidden units in first fully connected layer
- $N_{h2}$ : Number of hidden units in second fully connected layer
- *Batch norm*: Use of batch norm in the units
- *Residual units*: Use of residual units in the units

All evaluations are performed with a depth camera having a resolution of  $64 \times 64$  pixels. Here we note that we can not expect to achieve perfect prediction of the oracle’s target score as we have missing information and the predicted score is ambiguous. To demonstrate that we are learning a useful regressor we report both the normalized loss value (i.e. the loss on zero-mean and unit-variance target values) and the Spearman-correlation between predicted and target score.

#### 4.1 Input channels

In Table 1 we compare the performance of our model when using only the occupancy, only the uncertainty or both channels as input to the network. We use a basic configuration of  $N_c = 2$ ,  $N_u = 4$ ,  $N_f = 8$ ,  $L = 4$  and grid size of 16.

We note that using the occupancy channel performs better than using the uncertainty channel. However, using both channels together performs best. This can be explained by observing that the uncertainty channel carries no surface information and thus is less useful to reason about likely surface voxels. However, the uncertainty channel still carries orthogonal information. This makes intuitive sense as we can better reason about the utility of measurements if we know how uncertain we are about them. If we are certain about all the voxels there is not much to gain from a measurement.

| Loss for different input channels |       |       |
|-----------------------------------|-------|-------|
| Channels                          | Train | Test  |
| $v^o$                             | 0.261 | 0.212 |
| $v^u$                             | 0.305 | 0.258 |
| $v^o, v^u$                        | 0.272 | 0.207 |

  

| Spearman correlation for different input channels |       |       |
|---------------------------------------------------|-------|-------|
| Channels                                          | Train | Test  |
| $v^o$                                             | 0.869 | 0.917 |
| $v^u$                                             | 0.844 | 0.889 |
| $v^o, v^u$                                        | 0.870 | 0.926 |

Table 1: Comparison of loss and Spearman correlation between target score and predicted score for different input channels. The occupancy channel alone results in a lower loss than the uncertainty channel. However, using both channels results in the lowest loss and highest correlation. See main text for a more detailed discussion.

## 4.2 Input scales

In Table 2 we compare the performance of our model when using individual scales or using all scales as input to the network. We use a basic configuration of  $N_c = 2$ ,  $N_u = 4$ ,  $N_f = 8$ , both input channels and grid size of 16.

As we can see our network does not perform well when only using the first scale which only spans a region  $3.2m$  while our camera has a range of  $10m$ . On the other hand the second, third and fourth scale span a region of  $6.4$ ,  $12.8m$  and  $25.6m$  respectively and thus can provide a much more global view of the scene. Nevertheless, providing all scales as the input leads to a worse result than only providing scale the first 3 scales to the network. We hypothesize that this is due to a limited dataset size when considering the large spatial region of the fourth scale as there is an ever increasing number of configurations of the occupancy map depending on the viewpoint sequence.

| Loss for different scales |       |       |
|---------------------------|-------|-------|
| Scales                    | Train | Test  |
| 0                         | 0.476 | 0.444 |
| 1                         | 0.298 | 0.263 |
| 2                         | 0.257 | 0.212 |
| 3                         | 0.311 | 0.249 |
| 0, 1, 2                   | 0.271 | 0.189 |
| 0, 1, 2, 3                | 0.272 | 0.207 |

  

| Spearman correlation for different scales |       |       |
|-------------------------------------------|-------|-------|
| Scales                                    | Train | Test  |
| 0                                         | 0.721 | 0.756 |
| 1                                         | 0.831 | 0.873 |
| 2                                         | 0.871 | 0.926 |
| 3                                         | 0.844 | 0.900 |
| 0, 1, 2                                   | 0.864 | 0.930 |
| 0, 1, 2, 3                                | 0.870 | 0.926 |

Table 2: Comparison of loss and Spearman correlation between target score and predicted score for different input scales. Scale 2 and 3 give a much lower loss than scale 0 and 1. However, using scales 0, 1, 2 results in the lowest loss and highest correlation. See main text for a more detailed discussion.

## 4.3 Model architecture

We further evaluate the model architecture using a grid size of 16 with  $L = 3$  scales and both input channels (best configuration from previous evaluation).

We evaluate hyper-parameters individually using a base configuration of  $N_c = 2$ ,  $N_u = 4$ ,  $N_f = 8$ ,  $N_{h1} = 128$ ,  $N_{h2} = 32$ , no Batch-Norm and no residual units. The results are shown in Table 3 where the best hyperparameter settings are marked with an

asterisk. The *Residual unit* variant uses a residual unit as in [3] (without bottleneck). as the second unit in each block. Note that the result of the base configuration appears multiple times in the table.

For our final architecture we identify the best hyperparameters as  $N_c = 2$ ,  $N_u = 4$ ,  $N_f = 8$ ,  $N_{h1} = 128$ ,  $N_{h2} = 32$  and using Batch Norm.

| Loss for different architectures |       |       |
|----------------------------------|-------|-------|
| Grid size                        | Train | Test  |
| $N_u = 1$                        | 0.205 | 0.244 |
| $N_u = 2$                        | 0.211 | 0.239 |
| * $N_u = 3$                      | 0.173 | 0.179 |
| $N_f = 4$                        | 0.177 | 0.182 |
| * $N_f = 8$                      | 0.173 | 0.179 |
| $N_f = 16$                       | 0     | 0.197 |
| * Batch-Norm                     | 0.112 | 0.186 |
| Residual units                   | 0.190 | 0.206 |
| * FC [128, 32]                   | 0.173 | 0.179 |
| FC [256, 64]                     | 0.195 | 0.185 |
| FC [256, 128]                    | 0.273 | 0.197 |
| FC [512, 256]                    | 0.170 | 0.201 |

  

| Spearman correlation for different block sizes |        |       |
|------------------------------------------------|--------|-------|
| Channels                                       | Train  | Test  |
| $N_u = 1$                                      | 0.899  | 0.919 |
| $N_u = 2$                                      | 0.899  | 0.925 |
| * $N_u = 3$                                    | 0.918  | 0.932 |
| $N_f = 4$                                      | 0.919  | 0.931 |
| * $N_f = 8$                                    | 0.9180 | 0.932 |
| $N_f = 16$                                     | 0.920  | 0.928 |
| * Batch-Norm                                   | 0.940  | 0.942 |
| Residual units                                 | 0.912  | 0.929 |
| * FC [128, 32]                                 | 0.918  | 0.932 |
| FC [256, 64]                                   | 0.901  | 0.926 |
| FC [256, 128]                                  | 0.865  | 0.925 |
| FC [512, 256]                                  | 0.920  | 0.930 |

Table 3: Comparison of loss and Spearman correlation between target score and predicted score for different model variants. Individual hyperparameters with best performance are marked with an asterisk. See main text for a description.

#### 4.4 Grid size

In table Table 4 we show the results of using different grid sizes for the local multi-scale representation of the occupancy map. We use a basic configuration of  $N_c = 2$ ,  $N_u = 4$ ,  $N_f = 8$ ,  $N_{h1} = 128$ ,  $N_{h2} = 32$ , using Batch Norm and both input channels. We chose

the number of scales so that the total spatial extent of the representation is the same for all grid sizes.

We can see a general trend of a higher Spearman correlation with increasing grid size. However, with a grid size of 64 we see a lower correlation than with a grid size of 32. As we keep the number of samples in the dataset constant between grid sizes we hypothesize that the lower performance for a grid size of 64 is due to insufficient data compared to the much larger network and number of parameters. While the grid size of 32 gives the best performance we chose a grid size of 16 for all our exploration experiments. This is a tradeoff between performance and computation time. In particular the sampling of the occupancy map is about 8 times faster with grid size 16 as compared to grid size 32.

| Loss for different input grid sizes |       |       |
|-------------------------------------|-------|-------|
| Grid size                           | Train | Test  |
| 8                                   | 0.145 | 0.235 |
| 16                                  | 0.112 | 0.186 |
| 32                                  | 0.156 | 0.263 |
| 64                                  | 0.248 | 0.192 |

  

| Spearman correlation for different input grid sizes |       |       |
|-----------------------------------------------------|-------|-------|
| Channels                                            | Train | Test  |
| 8                                                   | 0.920 | 0.921 |
| 16                                                  | 0.912 | 0.942 |
| 32                                                  | 0.932 | 0.953 |
| 64                                                  | 0.835 | 0.950 |

Table 4: Comparison of loss and Spearman correlation between target score and predicted score for different input grid sizes. With larger grid sizes than 16 the Spearman correlation is higher but we already see that with a grid size of 64 the correlation is lower than with 32. We hypothesize that this is due to insufficient data compared to a much larger network and number of parameters. As a trade-off between performance and computation time we chose grid size 16 our main model. See main text for a more detailed discussion.

#### 4.5 Modified neighborhood movements

Here we report results of our model when using a different neighborhood of viewpoint poses. The motion distance is increased to  $6m$  and the rotation angle is increased to  $45^\circ$ . Results are shown in Fig. 3 for the scene *Washington1*. Our model outperforms the baselines despite using a neighborhood different from the one used to generate training data.

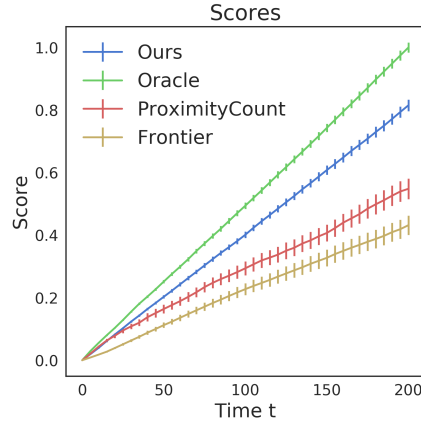

Fig. 3: Plot of observed surface voxels vs. time for all methods on the *Washington1* scene using a different viewpoint neighborhood than used when generating training data. Plots were computed across 50 explorations. Best viewed in color.

#### 4.6 Stereo data

An example of ground truth depth and depth from stereo data is shown in Fig. 4.

### 5 Visualization of multi-scale representation

In Fig. Fig. 5 we show visualizations of our multi-scale representation for a grid size of 16. Shown are horizontal slices of the 3D grid representation at a fixed height for random samples from the *Neighborhood* dataset. The multiscale representation allows us to get an idea about the surrounding of the camera pose: For example 1 there is a building at the lower right corner and on the larger scales we can even see that there is also a building in the upper left corner. For example 2 we only see a wall on the right side and the uncertainty plot in the bottom row shows us that most of the surrounding on the larger scales has not been explored yet. This is a good indication that our data is rich enough for our 3D ConvNet to learn general concepts about geometric structure and distribution and generalize to new scenes.

### 6 Details for training procedure

#### 6.1 Normalization and learning rate

We normalize input and target data to be zero-mean and unit-variance. Input data normalization is done per channel (i.e. occupancy and uncertainty for each scale) across all grid elements.

Training is done with a mini-batch size of 128, and a learning rate of  $r = 10^{-3}/(1 + 0.5e)$ , where  $e$  is the current epoch, starting at 0. We noticed only slight improvement in contrast to a constant learning rate of  $r = 10^{-3}$ .

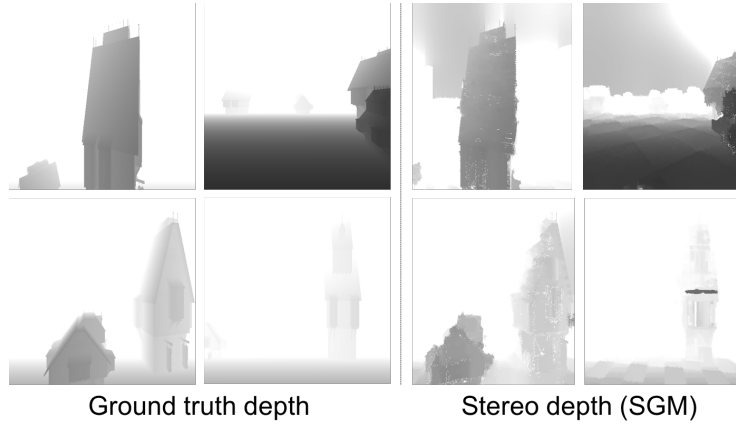

Fig. 4: To evaluate how our method handles noisy input such as depth images resulting from stereo cameras we compute depth images from a virtual stereo pair. Shown on the left are examples of ground truth depth image. On the right we show the corresponding depth images computed with semi-global matching [4] using a stereo baseline of  $0.5m$ .

## 6.2 Data augmentation

Due to our input representation we are not able to augment our data in a similar fashion as for image data. Our representation is directly related to an absolute scale and thus cropping and rescaling the grids is undesirable. This also prevents us from using rotations as we either have to crop and rescale the grids afterwards or pad the points without data with a constant value which would distort our data distribution. While we could use a dataset with bigger grid size (i.e. larger by a factor of  $\sqrt{3}$ ) to ensure that all rotations can be done without cropping we decided against this due to the unknown change in the data distribution caused by the required interpolation.

## 7 Relation between our method and POMDPs

Our problem can also be formulated as a Partially Observable Markov Decision Process POMDP. In this case the state space is given by the whole map and the camera pose. The map update and the pose-transition function are then describing the state-transition function in a generative form and the oracle score represents the reward signal.

Dynamic programming methods with Monte-Carlo sampling are able to handle large state spaces [5,6], however, these approaches are usually limited to problems with discrete state spaces and a discrete reward signal and require a complete model of the system dynamics. In our case both the state and the reward signal are continuous and we do not have a model of the complete system due to missing ground truth.

Contrary to this, reinforcement learning, using ConvNets as function approximators, has seen a huge success in learning policies on visual input data. Such problems include

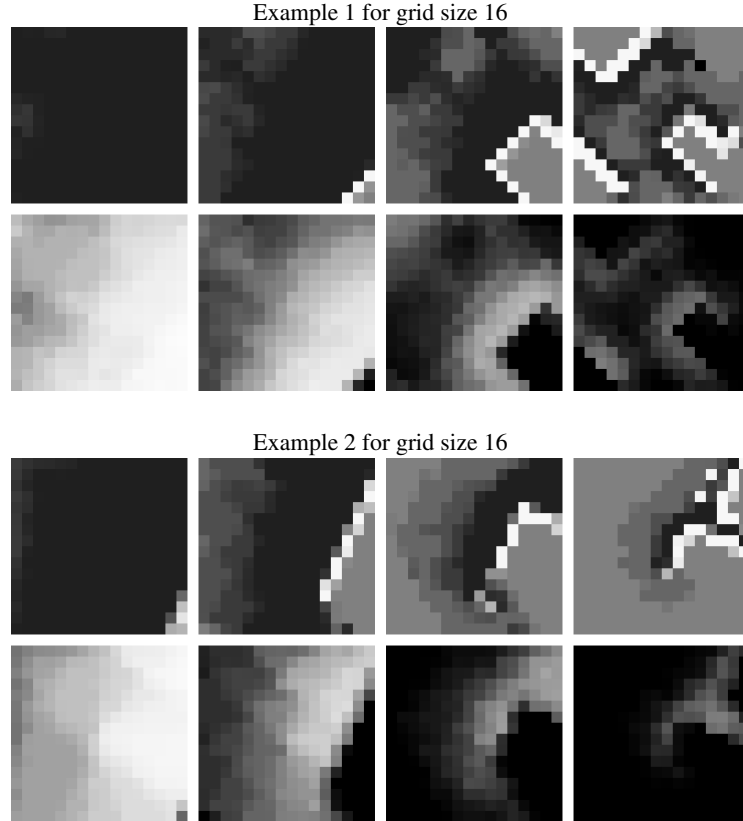

Fig. 5: Shown are horizontal slices of the 3D grid representation at a fixed height. The examples are random samples from the *Neighborhood* dataset (grid size 16 with  $L = 4$  scales). Top row: Occupancies. Bottom row: Certainties (i.e.  $1 - v^u$ ). Left column: Smallest scale. Right column: Largest scale. Black represents 0, white represents 1.

moving an agent to a goal position or scoring a high number of points in a video game. Usually, these problems can be run at step-rates well over  $1kH_z$ . Contrary to this, the steps in our problem are computationally expensive due to the map update and thus we are limited to step-rates on the order of  $20H_z$  thus making reinforcement learning in our current setting a very time-consuming and impractical undertaking.

## References

1. Hornung, A., Wurm, K.M., Bennewitz, M., Stachniss, C., Burgard, W.: OctoMap: An efficient probabilistic 3D mapping framework based on octrees. *Autonomous Robots* (2013) Software available at <http://octomap.github.com>.
2. Krause, A., Golovin, D.: Submodular function maximization. *Tractability: Practical Approaches to Hard Problems* (2012)
3. He, K., Zhang, X., Ren, S., Sun, J.: Deep residual learning for image recognition. In: *Proceedings of the IEEE conference on computer vision and pattern recognition*. (2016) 770–778
4. Hirschmuller, H.: Stereo processing by semiglobal matching and mutual information. *IEEE Transactions on pattern analysis and machine intelligence* **30**(2) (2008) 328–341
5. Silver, D., Veness, J.: Monte-carlo planning in large pomdps. In Lafferty, J.D., Williams, C.K.I., Shawe-Taylor, J., Zemel, R.S., Culotta, A., eds.: *Advances in Neural Information Processing Systems 23*. Curran Associates, Inc. (2010) 2164–2172
6. Somani, A., Ye, N., Hsu, D., Lee, W.S.: Despot: Online pomdp planning with regularization. In: *Advances in neural information processing systems*. (2013) 1772–1780
